# Supplementary material for: A Large-Scale Survey of Password Entry Practices on Non-Desktop Devices
Source: arXiv:2409.03044 source file (2024-09-04)
Supplement: Supplementary file 1 [file appendix-2.tex]

\section{Tables With Demographic Breakdown}

\subsection{Methodology}
\begin{table} [p]
	\caption{Demographics for the participants taking the study, less those that were removed for quality reasons.}
	\label{tab:demographics_breakdown}
	\begin{adjustbox}{max width=\textwidth}
		\begin{tabular}{llrrrr}
	\toprule
      &  & Overall (Overall \%) & EU (EU \%) & USA (USA \%) & UK (UK \%) \\
      \midrule
     Participants &  & 999 (100\%) & 601 (60\%) & 299 (30\%) & 99 (10\%) \\
     & & & & & \\
     \multirow[c]{3}{*}{Gender} & Male & 495 (50\%) & 300 (50\%) & 149 (50\%) & 46 (46\%) \\
      & Female & 486 (49\%) & 292 (49\%) & 144 (48\%) & 50 (51\%) \\
      & I prefer not to answer & 18 (2\%) & 9 (1\%) & 6 (2\%) & 3 (3\%) \\
      & & & & & \\
     \multirow[c]{6}{*}{Age} & 18-25 & 373 (37\%) & 282 (47\%) & 70 (23\%) & 21 (21\%) \\
      & 26-35 & 343 (34\%) & 205 (34\%) & 103 (34\%) & 35 (35\%) \\
      & 36-45 & 161 (16\%) & 83 (14\%) & 67 (22\%) & 11 (11\%) \\
      & 46-55 & 72 (7\%) & 22 (4\%) & 34 (11\%) & 16 (16\%) \\
      & 55+ & 47 (5\%) & 9 (1\%) & 24 (8\%) & 14 (14\%) \\
      & I prefer not to answer & 3 (0\%) & 0 (0\%) & 1 (0\%) & 2 (2\%) \\
      & & & & & \\
     \multirow[c]{9}{*}{Education} & Less than high school degree & 19 (2\%) & 12 (2\%) & 3 (1\%) & 4 (4\%) \\
      & High school graduate (high school diploma or equivalent including GED) & 184 (18\%) & 130 (22\%) & 41 (14\%) & 13 (13\%) \\
      & Some college but no degree & 191 (19\%) & 94 (16\%) & 73 (24\%) & 24 (24\%) \\
      & Associate's degree in college (2-year) & 55 (6\%) & 30 (5\%) & 20 (7\%) & 5 (5\%) \\
      & Bachelor's degree in college (4-year) & 337 (34\%) & 192 (32\%) & 109 (36\%) & 36 (36\%) \\
      & Master's degree & 172 (17\%) & 117 (19\%) & 41 (14\%) & 14 (14\%) \\
      & Doctoral degree & 15 (2\%) & 11 (2\%) & 3 (1\%) & 1 (1\%) \\
      & Professional degree (JD, MD) & 18 (2\%) & 9 (1\%) & 8 (3\%) & 1 (1\%) \\
      & I prefer not to answer & 8 (1\%) & 6 (1\%) & 1 (0\%) & 1 (1\%) \\
      \bottomrule
     \end{tabular}
	\end{adjustbox}
\end{table}

\subsection{Quantitative Results} 
\begin{table} [p]
	\caption{The list of devices and how many participants indicated using them to enter passwords.}
	\label{tab:device_usage_breakdown}
	\begin{adjustbox}{max width=\textwidth}
\begin{tabular}{llrrrr}
	\toprule
	&  & Overall (Overall \%) & EU (EU \%) & USA (USA \%) & UK (UK \%) \\
	\midrule
	\multirow[c]{7}{*}{General} &  & 997 (100\%) & 599 (100\%) & 299 (100\%) & 99 (100\%) \\
	& Phone & 980 (98\%) & 590 (98\%) & 291 (97\%) & 99 (100\%) \\
	& Laptop & 847 (85\%) & 499 (83\%) & 263 (88\%) & 85 (86\%) \\
	& Desktop & 644 (64\%) & 398 (66\%) & 189 (63\%) & 57 (58\%) \\
	& Tablet & 477 (48\%) & 254 (42\%) & 170 (57\%) & 53 (54\%) \\
	& Smartwatch & 127 (13\%) & 57 (9\%) & 58 (19\%) & 12 (12\%) \\
	& Smart speaker & 36 (4\%) & 19 (3\%) & 13 (4\%) & 4 (4\%) \\
	& & & & & \\
	\multirow[c]{5}{*}{Physical} &  & 862 (86\%) & 496 (83\%) & 270 (90\%) & 96 (97\%) \\
	& ATM & 819 (82\%) & 464 (77\%) & 262 (88\%) & 93 (94\%) \\
	& Physical keypad & 379 (38\%) & 194 (32\%) & 137 (46\%) & 48 (48\%) \\
	& Kiosk computer or tablet & 168 (17\%) & 69 (11\%) & 82 (27\%) & 17 (17\%) \\
	& Printer & 136 (14\%) & 72 (12\%) & 37 (12\%) & 27 (27\%) \\
	& & & & & \\
	\multirow[c]{6}{*}{Smart} &  & 570 (57\%) & 320 (53\%) & 187 (63\%) & 63 (64\%) \\
	& TV / Smart TV & 416 (42\%) & 238 (40\%) & 127 (42\%) & 51 (52\%) \\
	& Security alarm & 165 (17\%) & 78 (13\%) & 68 (23\%) & 19 (19\%) \\
	& Lock / Smart lock & 141 (14\%) & 75 (12\%) & 58 (19\%) & 8 (8\%) \\
	& Safe / Smart safe & 112 (11\%) & 55 (9\%) & 47 (16\%) & 10 (10\%) \\
	& Thermostat / Smart thermostat & 34 (3\%) & 12 (2\%) & 17 (6\%) & 5 (5\%) \\
	& & & & & \\
	\multirow[c]{7}{*}{Gaming} &  & 447 (45\%) & 246 (41\%) & 158 (53\%) & 43 (43\%) \\
	& PlayStation & 265 (27\%) & 147 (24\%) & 91 (30\%) & 27 (27\%) \\
	& Xbox & 180 (18\%) & 88 (15\%) & 77 (26\%) & 15 (15\%) \\
	& Nintendo Switch & 178 (18\%) & 85 (14\%) & 80 (27\%) & 13 (13\%) \\
	& VR headset & 36 (4\%) & 16 (3\%) & 19 (6\%) & 1 (1\%) \\
	& Other game console & 23 (2\%) & 13 (2\%) & 9 (3\%) & 1 (1\%) \\
	& Steam Deck & 22 (2\%) & 8 (1\%) & 10 (3\%) & 4 (4\%) \\
	& & & & & \\
	\multirow[c]{11}{*}{Other} &  & 101 (10\%) & 59 (10\%) & 29 (10\%) & 13 (13\%) \\
	& POS & 16 (2\%) & 12 (2\%) & 2 (1\%) & 2 (2\%) \\
	& Doors & 11 (1\%) & 5 (1\%) & 3 (1\%) & 3 (3\%) \\
	& Touchscreen tablet & 8 (1\%) & 4 (1\%) & 4 (1\%) & 0 (0\%) \\
	& Nintendo DS & 7 (1\%) & 6 (1\%) & 1 (0\%) & 0 (0\%) \\
	& Biometrics & 6 (1\%) & 3 (0\%) & 1 (0\%) & 2 (2\%) \\
	& Locker & 5 (1\%) & 4 (1\%) & 1 (0\%) & 0 (0\%) \\
	& Time Clock Machine & 5 (1\%) & 2 (0\%) & 0 (0\%) & 3 (3\%) \\
	& Gates & 5 (1\%) & 4 (1\%) & 1 (0\%) & 0 (0\%) \\
	& Safe & 5 (1\%) & 2 (0\%) & 3 (1\%) & 0 (0\%) \\
	& Car & 5 (1\%) & 0 (0\%) & 5 (2\%) & 0 (0\%) \\
	\bottomrule
\end{tabular}
	\end{adjustbox}
\end{table}

\subsection{Qualitative Results} 
\begin{table} [p]
	\caption{List of comments about virtual keyboards and how many participants indicated each comment.}
	\label{tab:virtual_comments_breakdown}
	\begin{adjustbox}{max width=\textwidth}
	\begin{tabular}{llrrrrr}
		\toprule
		Theme & Comment & Overall (Overall \%) & EU (EU \%) & USA (USA \%) & UK (UK \%) \\
		\midrule
		&Any Virtual Keyboard Comment & 421 (100.00\%) & 253 (100.00\%) & 123 (100.00\%) & 45 (100.00\%) \\
		\multirow[c]{6}{*}{Virtual Keyboards are Hard} & & \\
		&Virtual Keyboard Entry Hard & 56 (13.30\%) & 33 (13.04\%) & 17 (13.82\%) & 6 (13.33\%) \\
		&Mobile Entry Hard & 65 (15.44\%) & 42 (16.60\%) & 15 (12.20\%) & 8 (17.78\%) \\
		&Mobile Entry Slow & 14 (3.33\%) & 10 (3.95\%) & 3 (2.44\%) & 1 (2.22\%) \\
		&Touchscreen Entry Hard & 23 (5.46\%) & 15 (5.93\%) & 6 (4.88\%) & 2 (4.44\%) \\
		& & \\
		\multirow[c]{9}{*}{Controller Entry is Hard} & & \\
		&Game Entry Hard & 107 (25.42\%) & 60 (23.72\%) & 34 (27.64\%) & 13 (28.89\%) \\
		&Game Entry Slow & 38 (9.03\%) & 18 (7.11\%) & 15 (12.20\%) & 5 (11.11\%) \\
		&Game Arrow Key Entry Bad & 25 (5.94\%) & 13 (5.14\%) & 9 (7.32\%) & 3 (6.67\%) \\
		&Game Entry Uncomfortable & 4 (0.95\%) & 4 (1.58\%) & 0 (0.00\%) & 0 (0.00\%) \\
		&TV Entry Hard & 109 (25.89\%) & 62 (24.51\%) & 38 (30.89\%) & 9 (20.00\%) \\
		&TV Entry Slow & 109 (25.89\%) & 62 (24.51\%) & 38 (30.89\%) & 9 (20.00\%) \\
		&TV Arrow Key Entry Bad & 32 (7.60\%) & 14 (5.53\%) & 16 (13.01\%) & 2 (4.44\%) \\
		&TV Entry Uncomfortable & 2 (0.48\%) & 2 (0.79\%) & 0 (0.00\%) & 0 (0.00\%) \\
		& & \\
		\multirow[c]{5}{*}{Touchscreens May Be Better} & & \\
		&Touchscreen Entry Fast & 4 (0.95\%) & 2 (0.79\%) & 0 (0.00\%) & 2 (4.44\%) \\
		&Touchscreen Entry Easy & 35 (8.31\%) & 20 (7.91\%) & 9 (7.32\%) & 6 (13.33\%) \\
		&Mobile Entry Easy & 78 (18.53\%) & 47 (18.58\%) & 25 (20.33\%) & 6 (13.33\%) \\
		&Mobile Entry Fast & 13 (3.09\%) & 10 (3.95\%) & 1 (0.81\%) & 2 (4.44\%) \\
		\bottomrule
	\end{tabular}
\end{adjustbox}
\end{table}

\begin{table} [p]
	\caption{List of comments about virtual keyboard layout and how many participants indicated each comment.}
	\label{tab:layout_comments_breakdown}
	\begin{adjustbox}{max width=\textwidth}
	\begin{tabular}{lllll}
		\toprule
		Comment & Overall (Overall \%) & EU (EU \%) & USA (USA \%) & UK (UK \%) \\
		\midrule
		Any Virtual Keyboard Comment & 421 (100.00\%) & 253 (100.00\%) & 123 (100.00\%) & 45 (100.00\%) \\
		Special Characters Hard to Use & 35 (8.31\%) & 21 (8.30\%) & 10 (8.13\%) & 4 (8.89\%) \\
		Layout Switching Hard & 20 (4.75\%) & 13 (5.14\%) & 4 (3.25\%) & 3 (6.67\%) \\
		Virtual Keyboard Layout Matters & 22 (5.23\%) & 15 (5.93\%) & 6 (4.88\%) & 1 (2.22\%) \\
		Familiarity Matters & 43 (10.21\%) & 28 (11.07\%) & 11 (8.94\%) & 4 (8.89\%) \\
		\bottomrule
	\end{tabular}
\end{adjustbox}
\end{table}

\begin{table} [p]
	\caption{List of comments about physical devices and how many participants indicated each comment.}
	\label{tab:pc_comments_breakdown}
	\begin{adjustbox}{max width=\textwidth}
		\begin{tabular}{lllll}
			\toprule
			Comment & Overall (Overall \%) & EU (EU \%) & USA (USA \%) & UK (UK \%) \\
			\midrule
			Any Physical Entry Comment & 271 (100.00\%) & 176 (100.00\%) & 68 (100.00\%) & 27 (100.00\%) \\
			Physical Entry Easy & 221 (81.55\%) & 141 (80.11\%) & 59 (86.76\%) & 21 (77.78\%) \\
			Physical Entry Hard & 10 (3.69\%) & 7 (3.98\%) & 2 (2.94\%) & 1 (3.70\%) \\
			Physical Entry Fast & 47 (17.34\%) & 32 (18.18\%) & 9 (13.24\%) & 6 (22.22\%) \\
			Physical Entry Comfortable & 8 (2.95\%) & 8 (4.55\%) & 0 (0.00\%) & 0 (0.00\%) \\
			Physical Entry Less Mistakes & 5 (1.85\%) & 4 (2.27\%) & 0 (0.00\%) & 1 (3.70\%) \\
			\bottomrule
		\end{tabular}
	\end{adjustbox}
\end{table}

\begin{table} [p]
	\caption{List of comments about speed and how many participants indicated each comment.}
	\label{tab:speed_comments_breakdown}
	\begin{adjustbox}{max width=\textwidth}
		\begin{tabular}{lllll}
			\toprule
			Comment & Overall (Overall \%) & EU (EU \%) & USA (USA \%) & UK (UK \%) \\
			\midrule
			Any Speed Comment & 143 (100.00\%) & 91 (100.00\%) & 38 (100.00\%) & 14 (100.00\%) \\
			Physical Entry Fast & 47 (32.87\%) & 32 (35.16\%) & 9 (23.68\%) & 6 (42.86\%) \\
			Physical Entry Slow & 0 (0.00\%) & 0 (0.00\%) & 0 (0.00\%) & 0 (0.00\%) \\
			Mobile Entry Fast & 13 (9.09\%) & 10 (10.99\%) & 1 (2.63\%) & 2 (14.29\%) \\
			Mobile Entry Slow & 14 (9.79\%) & 10 (10.99\%) & 3 (7.89\%) & 1 (7.14\%) \\
			Touchscreen Entry Fast & 4 (2.80\%) & 2 (2.20\%) & 0 (0.00\%) & 2 (14.29\%) \\
			Touchscreen Entry Slow & 3 (2.10\%) & 2 (2.20\%) & 1 (2.63\%) & 0 (0.00\%) \\
			Game Entry Fast & 0 (0.00\%) & 0 (0.00\%) & 0 (0.00\%) & 0 (0.00\%) \\
			Game Entry Slow & 38 (26.57\%) & 18 (19.78\%) & 15 (39.47\%) & 5 (35.71\%) \\
			TV Entry Fast & 0 (0.00\%) & 0 (0.00\%) & 0 (0.00\%) & 0 (0.00\%) \\
			TV Entry Slow & 42 (29.37\%) & 24 (26.37\%) & 14 (36.84\%) & 4 (28.57\%) \\
			\bottomrule
		\end{tabular}
	\end{adjustbox}
\end{table}

\begin{table} [p]
	\caption{List of comments about cross-device considerations and how many participants indicated each comment.}
	\label{tab:cross_device_comments_breakdown}
	\begin{adjustbox}{max width=\textwidth}
		\begin{tabular}{lllll}
			\toprule
			Comment & Overall (Overall \%) & EU (EU \%) & USA (USA \%) & UK (UK \%) \\
			\midrule
			Devices Has Impact & 855 (85.59\%) & 523 (87.02\%) & 249 (83.28\%) & 83 (83.84\%) \\
			Device Has No Impact & 53 (5.31\%) & 32 (5.32\%) & 15 (5.02\%) & 6 (6.06\%) \\
			Comfort Matters & 11 (1.10\%) & 11 (1.83\%) & 0 (0.00\%) & 0 (0.00\%) \\
			Device Size Matters & 69 (6.91\%) & 42 (6.99\%) & 17 (5.69\%) & 10 (10.10\%) \\
			Mistakes Matter & 57 (5.71\%) & 37 (6.16\%) & 14 (4.68\%) & 6 (6.06\%) \\
			Mistakes Cause Challenges & 74 (7.41\%) & 51 (8.49\%) & 17 (5.69\%) & 6 (6.06\%) \\
			Frequency of Authentication Matters & 12 (1.20\%) & 7 (1.16\%) & 5 (1.67\%) & 0 (0.00\%) \\
			Security Matters & 83 (8.31\%) & 66 (10.98\%) & 8 (2.68\%) & 9 (9.09\%) \\
			\bottomrule
		\end{tabular}
	\end{adjustbox}
\end{table}

\begin{table} [p]
	\caption{List of comments about passwords and how many participants indicated each comment.}
	\label{tab:password_comments_breakdown}
	\begin{adjustbox}{max width=\textwidth}
		\begin{tabular}{lllll}
			\toprule
			Comment & Overall (Overall \%) & EU (EU \%) & USA (USA \%) & UK (UK \%) \\
			\midrule
			Any Password Comment & 340 (100.00\%) & 180 (100.00\%) & 118 (100.00\%) & 42 (100.00\%) \\
			Remembering Passwords Hard & 250 (73.53\%) & 127 (70.56\%) & 88 (74.58\%) & 35 (83.33\%) \\
			Creating New Passwords Hard & 24 (7.06\%) & 15 (8.33\%) & 7 (5.93\%) & 2 (4.76\%) \\
			Creating Unique Passwords Hard & 50 (14.71\%) & 19 (10.56\%) & 24 (20.34\%) & 7 (16.67\%) \\
			PCP Requirements Bad & 76 (22.35\%) & 36 (20.00\%) & 30 (25.42\%) & 10 (23.81\%) \\
			\bottomrule
		\end{tabular}
	\end{adjustbox}
\end{table}

\begin{table} [p]
\caption{List of other comments about passwords and how many participants indicated each comment.}
\label{tab:password_misc_comments_breakdown}
\begin{adjustbox}{max width=\textwidth}
	\begin{tabular}{lllll}
		\toprule
		Comment & Overall (Overall \%) & EU (EU \%) & USA (USA \%) & UK (UK \%) \\
		\midrule
		Any Password Lifecycle or Hardware Comment & 405 (100.00\%) & 223 (100.00\%) & 136 (100.00\%) & 46 (100.00\%) \\
		Hardware Doesn't Always Work & 59 (14.57\%) & 37 (16.59\%) & 19 (13.97\%) & 3 (6.52\%) \\
		Authentication Frequency High & 12 (2.96\%) & 7 (3.14\%) & 5 (3.68\%) & 0 (0.00\%) \\
		Password Forced Reset & 24 (5.93\%) & 15 (6.73\%) & 7 (5.15\%) & 2 (4.35\%) \\
		Password Recovery Hard & 16 (3.95\%) & 8 (3.59\%) & 6 (4.41\%) & 2 (4.35\%) \\
		Account Lockout Frustrating & 6 (1.48\%) & 3 (1.35\%) & 2 (1.47\%) & 1 (2.17\%) \\
		\bottomrule
	\end{tabular}
\end{adjustbox}
\end{table}

\begin{table} [p]
	\caption{List of comments about usability and how many participants indicated each comment.}
	\label{tab:usability_comments_breakdown}
	\begin{adjustbox}{max width=\textwidth}
		\begin{tabular}{lllll}
			\toprule
			Comment & Overall (Overall \%) & EU (EU \%) & USA (USA \%) & UK (UK \%) \\
			\midrule
			Any Usability Impacts Comment & 60 (100.00\%) & 28 (100.00\%) & 26 (100.00\%) & 6 (100.00\%) \\
			Usability Impacts Length & 28 (46.67\%) & 13 (46.43\%) & 10 (38.46\%) & 5 (83.33\%) \\
			Usability Impacts Complexity & 35 (58.33\%) & 15 (53.57\%) & 17 (65.38\%) & 3 (50.00\%) \\
			Usability Impacts Reuse & 1 (1.67\%) & 1 (3.57\%) & 0 (0.00\%) & 0 (0.00\%) \\
			Usability Impacts Usage & 6 (10.00\%) & 1 (3.57\%) & 5 (19.23\%) & 0 (0.00\%) \\
			\bottomrule
		\end{tabular}
	\end{adjustbox}
\end{table}

\begin{table} [p]
	\caption{List of comments about password managers and how many participants indicated each comment.}
	\label{tab:pwm_comments_breakdown}
	\begin{adjustbox}{max width=\textwidth}
		\begin{tabular}{lllll}
			\toprule
			Comment & Overall (Overall \%) & EU (EU \%) & USA (USA \%) & UK (UK \%) \\
			\midrule
			Uses Password Manager & 157 (15.72\%) & 89 (14.81\%) & 49 (16.39\%) & 19 (19.19\%) \\
			Wants Password Manager & 22 (2.20\%) & 7 (1.16\%) & 12 (4.01\%) & 3 (3.03\%) \\
			Password Manager Not Available & 67 (6.71\%) & 39 (6.49\%) & 21 (7.02\%) & 7 (7.07\%) \\
			Password Manager Syncing Issues & 6 (0.60\%) & 2 (0.33\%) & 3 (1.00\%) & 1 (1.01\%) \\
			Distrusts Password Manager & 17 (1.70\%) & 14 (2.33\%) & 2 (0.67\%) & 1 (1.01\%) \\
			\bottomrule
		\end{tabular}
	\end{adjustbox}
\end{table}

\begin{table} [p]
	\caption{List of comments about biometrics and how many participants indicated each comment.}
	\label{tab:bio_comments_breakdown}
	\begin{adjustbox}{max width=\textwidth}
		\begin{tabular}{lllll}
			\toprule
			Comment & Overall (Overall \%) & EU (EU \%) & USA (USA \%) & UK (UK \%) \\
			\midrule
			Prefers Biometrics & 242 (24.22\%) & 152 (25.29\%) & 63 (21.07\%) & 27 (27.27\%) \\
			Biometrics Not Available & 58 (5.81\%) & 29 (4.83\%) & 22 (7.36\%) & 7 (7.07\%) \\
			Biometrics Inaccurate & 117 (11.71\%) & 78 (12.98\%) & 30 (10.03\%) & 9 (9.09\%) \\
			Distrusts Biometrics & 16 (1.60\%) & 10 (1.66\%) & 4 (1.34\%) & 2 (2.02\%) \\
			Dislikes Biometrics & 2 (0.20\%) & 2 (0.33\%) & 0 (0.00\%) & 0 (0.00\%) \\
			\bottomrule
		\end{tabular}
	\end{adjustbox}
\end{table}

\begin{table} [p]
	\caption{List of comments about multi-factor authentication and how many participants indicated each comment.}
	\label{tab:mfa_comments_breakdown}
	\begin{adjustbox}{max width=\textwidth}
		\begin{tabular}{lllll}
			\toprule
			Comment & Overall (Overall \%) & EU (EU \%) & USA (USA \%) & UK (UK \%) \\
			\midrule
			Prefers Multi-Factor Authentication & 25 (2.50\%) & 12 (2.00\%) & 12 (4.01\%) & 1 (1.01\%) \\
			Multi-Factor Unavailable & 4 (0.40\%) & 4 (0.67\%) & 0 (0.00\%) & 0 (0.00\%) \\
			Distrusts Multi-Factor & 1 (0.10\%) & 0 (0.00\%) & 1 (0.33\%) & 0 (0.00\%) \\
			Dislikes Multi-Factor & 46 (4.60\%) & 17 (2.83\%) & 25 (8.36\%) & 4 (4.04\%) \\
			\bottomrule
		\end{tabular}
	\end{adjustbox}
\end{table}
